# Supplementary material for: Few-shot Video-to-Video Synthesis
Source: arXiv:1910.12713 source file (2019-10-28)
Supplement: Supplementary file 1 [file supp_ours.tex]

\begin{figure}[t!]
 \begin{tabular}{cc}
 \includegraphics[width=.45\hsize]{figures_supp/arch_ours_2.JPG}&
 \includegraphics[width=.45\hsize]{figures_supp/arch_ours_3.JPG}\\
 (a) & (b)
 \end{tabular}
 \vspace{-2mm}
  \caption{Details of our intermediate image synthesis network. (a) The figure visualizes that our network weight generation network $E$ converts the set of input example images and their corresponding semantic images to the network weights for a SPADE module (or a spatial modulation module) in the SPADE generator. (b) The figure visualizes that our network weight generation network $E$ generates the weights for all the SPADE modules in the SPADE generator.}
 \label{fig::supp_ours}
\end{figure}
